# Supplementary material for: Detailed Analysis of the NGC 2168 Cluster, Leveraging Gaia DR3
Source: arXiv:2603.22410 source file (2026-03-23)
Supplement: Supplementary file 1 [file AppendixA.tex]

% Please add the following required packages to your document preamble:
% \usepackage{graphicx}
\begin{table}[]
\resizebox{\columnwidth}{!}{%
\begin{tabular}{llllllllllll}
Source              & RA      & DEC     & RV      & RV\_Error & Survey   & Source              & RA      & DEC     & RV     & RV\_Error & Survey   \\
3426290609695576064 & 92.4477 & 24.3857 & -5.16   & 1.35      & APOGEE   & 3426263809097220352 & 92.3161 & 24.2144 & -37.62 & 12.76     & Gaia DR3 \\
3426270406169408512 & 92.3157 & 24.3788 & -8.67   & 0.60      & APOGEE   & 3426263912176435200 & 92.3308 & 24.2193 & -6.24  & 11.76     & Gaia DR3 \\
3426307583406596608 & 92.3315 & 24.5285 & -7.37   & 0.47      & APOGEE   & 3426264225713369344 & 92.2685 & 24.2122 & -22.40 & 8.27      & Gaia DR3 \\
3426290751431315456 & 92.4029 & 24.3722 & -7.36   & 4.03      & APOGEE   & 3426264427572833664 & 92.2242 & 24.2219 & -13.22 & 11.16     & Gaia DR3 \\
3426265222145752064 & 92.3629 & 24.2292 & -15.74  & 0.84      & APOGEE   & 3426264496292309632 & 92.2439 & 24.2373 & -11.24 & 5.21      & Gaia DR3 \\
3426311569136380800 & 92.2136 & 24.5920 & -7.65   & 0.70      & APOGEE   & 3426264603670482944 & 92.2891 & 24.2239 & -13.32 & 8.36      & Gaia DR3 \\
3425535799257924608 & 92.7942 & 24.2934 & -7.17   & 1.09      & APOGEE   & 3426264668092930048 & 92.2771 & 24.2305 & -3.09  & 6.32      & Gaia DR3 \\
3425403823502917888 & 92.2634 & 23.8036 & -3.01   & 11.97     & Gaia DR3 & 3426264706749693184 & 92.2807 & 24.2480 & -12.67 & 12.91     & Gaia DR3 \\
3425404751215869184 & 92.1545 & 23.8343 & -11.77  & 8.84      & Gaia DR3 & 3426264981627601664 & 92.2536 & 24.2656 & -8.23  & 0.12      & Gaia DR3 \\
3425409385486487680 & 92.1162 & 23.9275 & -5.01   & 4.75      & Gaia DR3 & 3426264981627804672 & 92.2559 & 24.2635 & -11.80 & 5.69      & Gaia DR3 \\
3425485049925167872 & 92.4150 & 23.7765 & -19.71  & 11.51     & Gaia DR3 & 3426265015987334016 & 92.2764 & 24.2656 & -17.49 & 9.10      & Gaia DR3 \\
3425485221723613824 & 92.4533 & 23.8008 & -0.58   & 5.13      & Gaia DR3 & 3426265119066538624 & 92.2925 & 24.2893 & 26.69  & 13.76     & Gaia DR3 \\
3425487661264989056 & 92.5058 & 23.8972 & -12.16  & 5.42      & Gaia DR3 & 3426265355293202176 & 92.3861 & 24.2511 & -4.43  & 8.78      & Gaia DR3 \\
3425494288396607488 & 92.6058 & 23.9881 & 5.08    & 16.14     & Gaia DR3 & 3426265462663916032 & 92.3604 & 24.2498 & -5.70  & 9.54      & Gaia DR3 \\
3425497488149739648 & 92.5954 & 24.0938 & -24.98  & 7.96      & Gaia DR3 & 3426265492726674176 & 92.3400 & 24.2572 & -41.81 & 9.05      & Gaia DR3 \\
3425498342845743360 & 92.3248 & 23.8725 & 7.90    & 12.15     & Gaia DR3 & 3426265664523409792 & 92.3742 & 24.2816 & -5.60  & 5.62      & Gaia DR3 \\
3425499858971793408 & 92.2839 & 23.9518 & 8.87    & 6.26      & Gaia DR3 & 3426265664525396992 & 92.3760 & 24.2798 & 11.49  & 9.67      & Gaia DR3 \\
3425500679307943808 & 92.4381 & 23.9891 & -10.58  & 14.33     & Gaia DR3 & 3426266012419708544 & 92.4109 & 24.2943 & -21.55 & 9.38      & Gaia DR3 \\
3425503153209105408 & 92.2414 & 24.0035 & -24.63  & 15.74     & Gaia DR3 & 3426266214279218816 & 92.4192 & 24.3240 & -1.79  & 28.09     & Gaia DR3 \\
3425503737324659712 & 92.1906 & 23.9769 & -10.18  & 8.28      & Gaia DR3 & 3426266214281275136 & 92.4118 & 24.3285 & 6.28   & 16.71     & Gaia DR3 \\
3425504360097512704 & 92.2755 & 23.9825 & -11.89  & 5.83      & Gaia DR3 & 3426266283000688384 & 92.3404 & 24.2845 & 4.87   & 6.68      & Gaia DR3 \\
3425505768846775552 & 92.2219 & 24.0688 & -3.63   & 5.57      & Gaia DR3 & 3426266351718176256 & 92.3221 & 24.2898 & 1.16   & 12.74     & Gaia DR3 \\
3425505798908955904 & 92.2342 & 24.0586 & -5.35   & 19.47     & Gaia DR3 & 3426266424736577408 & 92.3613 & 24.3017 & -24.96 & 17.83     & Gaia DR3 \\
3425507967869993856 & 92.4049 & 24.0607 & -8.29   & 6.49      & Gaia DR3 & 3426266557876606080 & 92.3170 & 24.2928 & -21.13 & 11.20     & Gaia DR3 \\
3425508414546577408 & 92.4404 & 24.0885 & -18.31  & 9.36      & Gaia DR3 & 3426266596535284992 & 92.2916 & 24.3008 & -14.89 & 6.26      & Gaia DR3 \\
3425509720216584832 & 92.5816 & 24.1633 & -18.42  & 10.99     & Gaia DR3 & 3426266626596080896 & 92.2989 & 24.3091 & -5.97  & 24.39     & Gaia DR3 \\
3425510334394414464 & 92.5513 & 24.1416 & -7.38   & 11.45     & Gaia DR3 & 3426267073272677632 & 92.3558 & 24.3254 & -20.80 & 36.28     & Gaia DR3 \\
3425510510490565248 & 92.5737 & 24.1757 & -18.29  & 4.51      & Gaia DR3 & 3426267077571603584 & 92.3472 & 24.3269 & 16.40  & 12.05     & Gaia DR3 \\
3425510579210039296 & 92.5688 & 24.1907 & 5.84    & 9.48      & Gaia DR3 & 3426267111931337600 & 92.3551 & 24.3386 & -10.21 & 8.36      & Gaia DR3 \\
3425510677991795968 & 92.5208 & 24.1774 & -8.87   & 9.63      & Gaia DR3 & 3426267215010546432 & 92.3729 & 24.3509 & -50.49 & 13.90     & Gaia DR3 \\
3425510751008737920 & 92.5462 & 24.1893 & 35.18   & 8.99      & Gaia DR3 & 3426267279431105024 & 92.3579 & 24.3587 & -86.62 & 29.19     & Gaia DR3 \\
3425511025886704256 & 92.3958 & 24.0835 & -3.51   & 10.81     & Gaia DR3 & 3426267519949284352 & 92.2254 & 24.2553 & -36.31 & 10.21     & Gaia DR3 \\
3425511296467091712 & 92.3748 & 24.1062 & 16.70   & 17.99     & Gaia DR3 & 3426267524248250112 & 92.2341 & 24.2500 & -7.38  & 7.73      & Gaia DR3 \\
3425511743143688832 & 92.4081 & 24.1307 & -14.00  & 11.19     & Gaia DR3 & 3426267592967726336 & 92.2174 & 24.2672 & -1.16  & 10.25     & Gaia DR3 \\
3425511919241092480 & 92.4124 & 24.1573 & -3.26   & 5.34      & Gaia DR3 & 3426267730406692736 & 92.1693 & 24.2660 & -6.20  & 12.41     & Gaia DR3 \\
3425512808297968896 & 92.3477 & 24.1623 & -3.32   & 4.27      & Gaia DR3 & 3426267730406875776 & 92.1719 & 24.2629 & -42.79 & 6.98      & Gaia DR3 \\
3425512846952824960 & 92.3570 & 24.1687 & -8.30   & 27.26     & Gaia DR3 & 3426267829186927616 & 92.1870 & 24.2728 & -14.19 & 14.06     & Gaia DR3 \\
3425512911374788992 & 92.3480 & 24.1892 & -14.28  & 14.95     & Gaia DR3 & 3426267833485903232 & 92.1861 & 24.2693 & -4.93  & 6.86      & Gaia DR3 \\
3425513151895374208 & 92.4420 & 24.1554 & -9.42   & 10.67     & Gaia DR3 & 3426267863546664192 & 92.2016 & 24.2906 & -19.05 & 26.06     & Gaia DR3 \\
3425513224909920000 & 92.4889 & 24.1589 & 10.93   & 11.92     & Gaia DR3 & 3426267863546664832 & 92.2065 & 24.2855 & -19.86 & 7.62      & Gaia DR3 \\
3425513843385190528 & 92.5226 & 24.2114 & 4.08    & 7.85      & Gaia DR3 & 3426268035345356544 & 92.2545 & 24.2866 & -24.80 & 35.78     & Gaia DR3 \\
3425514255703294720 & 92.4113 & 24.1960 & -20.55  & 6.53      & Gaia DR3 & 3426268074004040832 & 92.2710 & 24.2977 & -14.16 & 11.75     & Gaia DR3 \\
3425514358781283328 & 92.4392 & 24.2145 & -15.52  & 6.40      & Gaia DR3 & 3426268172786308608 & 92.2293 & 24.2859 & -10.89 & 9.88      & Gaia DR3 \\
3425514427501983488 & 92.4427 & 24.2258 & -9.77   & 8.31      & Gaia DR3 & 3426268177083271808 & 92.2206 & 24.2890 & -11.81 & 6.08      & Gaia DR3 \\
3425514530579986432 & 92.3852 & 24.2201 & -12.03  & 7.65      & Gaia DR3 & 3426268383241691648 & 92.2312 & 24.3130 & -7.14  & 8.45      & Gaia DR3 \\
3425515110401080448 & 92.4432 & 24.2626 & -6.81   & 7.54      & Gaia DR3 & 3426268482022160384 & 92.1614 & 24.2813 & -30.15 & 8.54      & Gaia DR3 \\
3425515213480279296 & 92.4540 & 24.2805 & 5.76    & 13.60     & Gaia DR3 & 3426268520677780096 & 92.1410 & 24.2828 & -37.47 & 14.14     & Gaia DR3 \\
3425534562307393664 & 92.6429 & 24.2355 & -29.33  & 10.77     & Gaia DR3 & 3426268653820645632 & 92.1616 & 24.2985 & -13.06 & 10.47     & Gaia DR3 \\
3425536177215079936 & 92.6820 & 24.2691 & -50.05  & 11.88     & Gaia DR3 & 3426268859979075584 & 92.1555 & 24.3007 & -13.77 & 14.83     & Gaia DR3 \\
3425536344719375360 & 92.7162 & 24.2889 & -6.69   & 14.34     & Gaia DR3 & 3426269036076728832 & 92.2007 & 24.3138 & -11.31 & 8.96      & Gaia DR3 \\
3425536619597362816 & 92.6965 & 24.3121 & -3.75   & 9.06      & Gaia DR3 & 3426269134856979328 & 92.2203 & 24.3290 & -6.38  & 8.63      & Gaia DR3 \\
3425536967489025408 & 92.7432 & 24.3526 & -7.77   & 22.85     & Gaia DR3 & 3426269207875413888 & 92.1996 & 24.3363 & -9.47  & 9.86      & Gaia DR3 \\
3425537581666932608 & 92.5393 & 24.2485 & -14.43  & 4.51      & Gaia DR3 & 3426269448393573120 & 92.2152 & 24.3571 & 4.53   & 8.11      & Gaia DR3 \\
3425538135720179584 & 92.5843 & 24.3033 & -9.07   & 13.03     & Gaia DR3 & 3426269448393574272 & 92.2096 & 24.3578 & -26.50 & 6.58      & Gaia DR3 \\
3425538307518870272 & 92.5829 & 24.3091 & -8.15   & 12.08     & Gaia DR3 & 3426269547173842560 & 92.2828 & 24.3053 & -20.71 & 21.28     & Gaia DR3 \\
3425538376238375296 & 92.5117 & 24.2640 & -33.08  & 7.34      & Gaia DR3 & 3426269585832518656 & 92.2976 & 24.3165 & 29.09  & 30.46     & Gaia DR3 \\
3425538479317586432 & 92.5073 & 24.2813 & 0.56    & 10.67     & Gaia DR3 & 3426269723271460608 & 92.3213 & 24.3380 & 0.69   & 1.79      & Gaia DR3 \\
3425538925994169344 & 92.5477 & 24.3105 & 3.10    & 9.41      & Gaia DR3 & 3426269890773286784 & 92.2453 & 24.3379 & 5.37   & 6.89      & Gaia DR3 \\
3425539711973732992 & 92.6512 & 24.3487 & -12.59  & 7.02      & Gaia DR3 & 3426270066868843520 & 92.2824 & 24.3755 & -11.14 & 3.51      & Gaia DR3 \\
3425539956786290944 & 92.6242 & 24.3548 & 15.64   & 8.78      & Gaia DR3 & 3426270204307787392 & 92.3363 & 24.3692 & -4.61  & 10.35     & Gaia DR3 \\
3425540777125620864 & 92.5998 & 24.3736 & 9.25    & 23.17     & Gaia DR3 & 3426270273027256960 & 92.3601 & 24.3804 & -12.40 & 2.44      & Gaia DR3 \\
3426158500798362624 & 91.8838 & 23.8599 & -12.31  & 37.86     & Gaia DR3 & 3426270307387001088 & 92.3336 & 24.3789 & -0.05  & 8.40      & Gaia DR3 \\
3426158805736491648 & 91.8840 & 23.8880 & -16.36  & 4.43      & Gaia DR3 & 3426270440527081088 & 92.2958 & 24.3805 & -3.49  & 4.21      & Gaia DR3 \\
3426159767812523904 & 92.0501 & 23.9270 & 195.78  & 13.38     & Gaia DR3 & 3426270440527081344 & 92.2901 & 24.3782 & 12.54  & 6.38      & Gaia DR3 \\
3426160523726752256 & 92.0513 & 23.9787 & -25.49  & 7.70      & Gaia DR3 & 3426270543606295168 & 92.3357 & 24.3933 & -6.08  & 11.73     & Gaia DR3 \\
3426161176561781120 & 91.9577 & 23.9898 & -6.33   & 4.29      & Gaia DR3 & 3426270784124417792 & 92.2622 & 24.3648 & -15.93 & 10.68     & Gaia DR3 \\
3426164101435660800 & 91.9326 & 24.0081 & 11.28   & 9.97      & Gaia DR3 & 3426270784124418304 & 92.2646 & 24.3597 & 0.62   & 7.08      & Gaia DR3 \\
3426164341954234368 & 91.9027 & 24.0096 & -12.22  & 11.47     & Gaia DR3 & 3426270788423355136 & 92.2591 & 24.3743 & -14.91 & 6.43      & Gaia DR3 \\
3426164956133180800 & 91.9832 & 24.0625 & -15.47  & 6.71      & Gaia DR3 & 3426270887203679488 & 92.2720 & 24.3876 & -7.56  & 21.04     & Gaia DR3 \\
3426165578904396800 & 91.8819 & 24.0690 & -9.48   & 10.31     & Gaia DR3 & 3426270925862316800 & 92.2257 & 24.3693 & -9.75  & 10.68     & Gaia DR3 \\
3426175749386993536 & 91.8165 & 24.0515 & -25.53  & 8.23      & Gaia DR3 & 3426270990284957056 & 92.2102 & 24.3751 & -29.72 & 13.30     & Gaia DR3 \\
3426181624901595392 & 91.7696 & 24.1509 & -4.68   & 12.11     & Gaia DR3 & 3426271093362107264 & 92.2520 & 24.4041 & -11.80 & 13.35     & Gaia DR3 \\
3426182346456026368 & 91.8129 & 24.2174 & -4.76   & 11.35     & Gaia DR3 & 3426271132020737536 & 92.2330 & 24.4025 & -17.58 & 20.70     & Gaia DR3 \\
3426230965485804672 & 91.7305 & 24.3125 & 0.19    & 6.63      & Gaia DR3 & 3426271196443425408 & 92.2868 & 24.3821 & -18.22 & 6.87      & Gaia DR3 \\
3426254909925014656 & 92.1579 & 24.0509 & -12.86  & 11.05     & Gaia DR3 & 3426271200740204288 & 92.2934 & 24.3903 & -24.48 & 10.00     & Gaia DR3 \\
3426255906357446912 & 92.1031 & 24.0781 & 9.05    & 5.37      & Gaia DR3 & 3426271200740205696 & 92.2887 & 24.3881 & -11.22 & 4.72      & Gaia DR3 \\
3426256009436612992 & 92.1199 & 24.0878 & -8.19   & 5.58      & Gaia DR3 & 3426271235099942144 & 92.2916 & 24.3946 & -10.89 & 8.51      & Gaia DR3 \\
3426256146875622400 & 92.0797 & 24.0868 & 5.67    & 8.58      & Gaia DR3 & 3426271338180113536 & 92.3038 & 24.4061 & -2.09  & 6.50      & Gaia DR3 \\
3426256563491758208 & 92.2076 & 24.0880 & 0.38    & 4.17      & Gaia DR3 & 3426271372538884864 & 92.3150 & 24.4194 & 2.26   & 2.59      & Gaia DR3 \\
3426256765350856960 & 92.1950 & 24.0971 & -17.88  & 3.20      & Gaia DR3 & 3426271372539132032 & 92.3164 & 24.4279 & -7.25  & 0.13      & Gaia DR3 \\
3426257108948444288 & 92.2599 & 24.1298 & -13.56  & 13.05     & Gaia DR3 & 3426271436959488896 & 92.3038 & 24.4240 & -0.99  & 6.51      & Gaia DR3 \\
3426258487637085312 & 92.1819 & 24.1972 & -8.46   & 9.44      & Gaia DR3 & 3426271647416788224 & 92.2968 & 24.4495 & -7.07  & 5.04      & Gaia DR3 \\
3426260033825377536 & 91.9556 & 24.1431 & -15.86  & 4.96      & Gaia DR3 & 3426272918726984192 & 91.8772 & 24.1906 & -12.82 & 8.13      & Gaia DR3 \\
3426260205624054912 & 92.0196 & 24.1406 & 9.50    & 13.31     & Gaia DR3 & 3426273227964614912 & 91.8694 & 24.2278 & -36.24 & 9.67      & Gaia DR3 \\
3426260824099321856 & 92.1062 & 24.1548 & -5.11   & 8.10      & Gaia DR3 & 3426273258025551744 & 91.8943 & 24.2255 & 11.92  & 21.82     & Gaia DR3 \\
3426260995898003712 & 92.1327 & 24.1774 & -10.84  & 8.87      & Gaia DR3 & 3426273777720394880 & 91.9087 & 24.2719 & -8.58  & 4.02      & Gaia DR3 \\
3426261472637256320 & 92.1895 & 24.2155 & -35.48  & 8.02      & Gaia DR3 & 3426273949519380736 & 92.0137 & 24.2238 & -13.74 & 7.17      & Gaia DR3 \\
3426261717452494208 & 92.1429 & 24.2251 & -6.00   & 5.87      & Gaia DR3 & 3426274185738693888 & 92.0439 & 24.2638 & 8.09   & 11.35     & Gaia DR3 \\
3426262439007001216 & 92.1233 & 24.2357 & 2.78    & 10.56     & Gaia DR3 & 3426278759882414464 & 91.9306 & 24.3442 & -5.31  & 16.38     & Gaia DR3 \\
3426262439007001728 & 92.1216 & 24.2353 & -10.81  & 9.51      & Gaia DR3 & 3426279103479758976 & 91.9928 & 24.3835 & -7.48  & 6.44      & Gaia DR3 \\
3426262473366746496 & 92.0940 & 24.2397 & -0.36   & 9.23      & Gaia DR3 & 3426279958175046656 & 91.8891 & 24.4173 & -9.67  & 3.35      & Gaia DR3 \\
3426263298000450176 & 92.2507 & 24.1668 & -3.18   & 9.87      & Gaia DR3 & 3426280271710883456 & 91.9136 & 24.4023 & 0.74   & 7.34      & Gaia DR3 \\
3426263396780601344 & 92.3014 & 24.1923 & -19.47  & 7.80      & Gaia DR3 & 3426280576649857920 & 92.1200 & 24.3114 & -16.69 & 12.91     & Gaia DR3 \\
Source              & RA      & DEC     & RV      & RV\_Error & Survey   & Source              & RA      & DEC     & RV     & RV\_Error & Survey   \\
3426280752747529344 & 92.1132 & 24.3350 & -28.33  & 7.74      & Gaia DR3 & 3426331330282114304 & 91.7700 & 24.4988 & -10.26 & 5.71      & Gaia DR3 \\
3426280782808284544 & 92.1222 & 24.3472 & -17.76  & 6.13      & Gaia DR3 & 3426336033267567616 & 92.0148 & 24.6114 & 3.14   & 9.09      & Gaia DR3 \\
3426280924545868544 & 92.0938 & 24.3462 & -20.12  & 22.40     & Gaia DR3 & 3426336445584427008 & 92.0466 & 24.6294 & -31.07 & 21.71     & Gaia DR3 \\
3426281126405667200 & 92.1709 & 24.3586 & -30.02  & 17.54     & Gaia DR3 & 3426336479944164864 & 92.0644 & 24.6379 & -30.81 & 13.06     & Gaia DR3 \\
3426281165064377984 & 92.1341 & 24.3566 & -7.55   & 9.38      & Gaia DR3 & 3426337102718017024 & 91.9687 & 24.6371 & -7.10  & 5.90      & Gaia DR3 \\
3426281298204405888 & 92.1675 & 24.3751 & -5.71   & 2.88      & Gaia DR3 & 3426338648906286720 & 91.8627 & 24.6384 & 2.32   & 7.49      & Gaia DR3 \\
3426281366923834752 & 92.1313 & 24.3647 & -15.55  & 4.30      & Gaia DR3 & 3426340504332087552 & 91.9926 & 24.6917 & -19.31 & 10.35     & Gaia DR3 \\
3426281783539323264 & 92.0841 & 24.3643 & -4.56   & 10.17     & Gaia DR3 & 3426361704290607872 & 92.0792 & 24.7545 & -13.17 & 12.95     & Gaia DR3 \\
3426282294636815616 & 92.1087 & 24.4011 & -18.05  & 33.92     & Gaia DR3 & 3426361841729552768 & 92.0908 & 24.7675 & -1.45  & 6.78      & Gaia DR3 \\
3426282298935369344 & 92.1053 & 24.4088 & -13.39  & 11.23     & Gaia DR3 & 3426363422277492096 & 92.1534 & 24.7888 & -1.97  & 4.54      & Gaia DR3 \\
3426282363356740992 & 92.1383 & 24.4161 & -13.18  & 6.84      & Gaia DR3 & 3426364796667052032 & 92.0859 & 24.7723 & -5.29  & 14.23     & Gaia DR3 \\
3426282779972048896 & 92.2070 & 24.4069 & -0.11   & 11.22     & Gaia DR3 & 3426257074588708480 & 92.2811 & 24.1364 & -9.21  & 2.45      & LAMOST   \\
3426282814331796096 & 92.1795 & 24.3952 & -15.21  & 9.71      & Gaia DR3 & 3426271024642633088 & 92.2225 & 24.3846 & -2.73  & 2.20      & LAMOST   \\
3426283054850806272 & 92.1819 & 24.4205 & -14.52  & 5.78      & Gaia DR3 & 3426282711252203392 & 92.1097 & 24.4599 & -8.87  & 3.02      & LAMOST   \\
3426283707684565760 & 92.2348 & 24.4723 & -12.69  & 31.87     & Gaia DR3 & 3426270543608387584 & 92.3452 & 24.3967 & -4.40  & 0.78      & LAMOST   \\
3426283772107799040 & 92.2329 & 24.4767 & -8.87   & 6.91      & Gaia DR3 & 3426297107982880768 & 92.4064 & 24.5199 & 1.74   & 1.19      & LAMOST   \\
3426283913843042816 & 92.1410 & 24.4402 & 2.79    & 8.17      & Gaia DR3 & 3426315524802189312 & 92.2607 & 24.7464 & -12.33 & 0.54      & LAMOST   \\
3426284051281979520 & 92.1661 & 24.4532 & 3.04    & 5.63      & Gaia DR3 & 3425539162218066432 & 92.5696 & 24.3403 & -11.28 & 1.25      & LAMOST   \\
3426284394879346304 & 92.1939 & 24.4724 & -11.34  & 10.59     & Gaia DR3 & 3426265458366936832 & 92.3688 & 24.2587 & -7.95  & 0.58      & LAMOST   \\
3426284463598819712 & 92.1900 & 24.4849 & -8.21   & 12.42     & Gaia DR3 & 3425514045248751360 & 92.5054 & 24.2286 & 2.00   & 1.05      & LAMOST   \\
3426284601037760896 & 92.2116 & 24.5007 & -8.90   & 0.12      & Gaia DR3 & 3425507418114160896 & 92.4855 & 24.0610 & -2.17  & 2.58      & LAMOST   \\
3426284905977634688 & 92.1902 & 24.5324 & 4.21    & 6.38      & Gaia DR3 & 3426230415730035712 & 91.6844 & 24.2803 & -17.31 & 2.85      & LAMOST   \\
3426284940336623104 & 92.0166 & 24.3866 & -51.60  & 20.33     & Gaia DR3 & 3426258895654696576 & 91.9817 & 24.0953 & -5.88  & 0.49      & LAMOST   \\
3426285352653482624 & 92.0200 & 24.4274 & -24.50  & 19.14     & Gaia DR3 & 3426263602939041152 & 92.3349 & 24.2049 & 12.43  & 3.09      & LAMOST   \\
3426285352653482752 & 92.0172 & 24.4255 & 2.66    & 7.24      & Gaia DR3 & 3426309301393630080 & 92.4091 & 24.5842 & 8.36   & 2.80      & LAMOST   \\
3426285460031314048 & 92.0179 & 24.4553 & -41.96  & 19.74     & Gaia DR3 & 3426292297619487104 & 92.5979 & 24.4608 & -3.90  & 2.38      & LAMOST   \\
3426285631829974528 & 92.0927 & 24.4539 & -2.91   & 13.71     & Gaia DR3 & 3426269929429902976 & 92.2608 & 24.3457 & 27.86  & 2.61      & LAMOST   \\
3426285631829976320 & 92.0867 & 24.4551 & -30.63  & 8.76      & Gaia DR3 & 3426295763656556288 & 92.3414 & 24.5118 & -5.12  & 1.92      & LAMOST   \\
3426285734909184384 & 92.0905 & 24.4672 & -4.24   & 16.94     & Gaia DR3 & 3426336209364790144 & 92.0854 & 24.6105 & -4.71  & 2.44      & LAMOST   \\
3426285803628677760 & 92.0595 & 24.4599 & -2.14   & 4.83      & Gaia DR3 & 3426263194921214592 & 92.3130 & 24.1843 & -8.58  & 2.25      & LAMOST   \\
3426285941067612416 & 92.0731 & 24.4864 & -10.18  & 11.69     & Gaia DR3 & 3426281886618521728 & 92.0968 & 24.3883 & -6.36  & 0.51      & LAMOST   \\
3426285941067614848 & 92.0793 & 24.4767 & -5.81   & 11.86     & Gaia DR3 & 3426282947478314752 & 92.2047 & 24.4258 & -2.15  & 2.89      & LAMOST   \\
3426286422104004992 & 91.9616 & 24.4714 & -12.49  & 7.83      & Gaia DR3 & 3425533290997088128 & 92.6312 & 24.1864 & -13.33 & 2.90      & LAMOST   \\
3426286903140306176 & 92.0080 & 24.5051 & -29.98  & 9.41      & Gaia DR3 & 3425510957167241088 & 92.3556 & 24.0677 & -10.50 & 1.61      & LAMOST   \\
3426287246737651840 & 92.1076 & 24.4973 & -15.87  & 6.94      & Gaia DR3 & 3426277626011130624 & 91.7793 & 24.3012 & -3.30  & 3.11      & LAMOST   \\
3426287276798871424 & 92.1332 & 24.4864 & -37.08  & 17.87     & Gaia DR3 & 3426289578903387136 & 92.4801 & 24.3532 & -6.24  & 0.62      & LAMOST   \\
3426287826555406208 & 92.1759 & 24.5394 & 2.87    & 5.32      & Gaia DR3 & 3426280409149815808 & 91.9362 & 24.4362 & -1.34  & 3.53      & LAMOST   \\
3426288483688221824 & 92.0864 & 24.5442 & -16.04  & 17.05     & Gaia DR3 & 3426259548489659904 & 92.0821 & 24.1528 & -11.43 & 3.04      & LAMOST   \\
3426289029145522432 & 92.1308 & 24.6006 & -0.15   & 7.17      & Gaia DR3 & 3426271269459685120 & 92.2668 & 24.3967 & -7.27  & 0.66      & LAMOST   \\
3426290236035226112 & 92.4740 & 24.3737 & -8.83   & 6.69      & Gaia DR3 & 3426284802900009728 & 92.1975 & 24.5069 & -5.26  & 1.35      & LAMOST   \\
3426290403535070848 & 92.5063 & 24.4013 & -20.47  & 14.91     & Gaia DR3 & 3426269993852533888 & 92.2958 & 24.3643 & -4.06  & 0.71      & LAMOST   \\
3426290437894766208 & 92.4125 & 24.3475 & -10.43  & 19.11     & Gaia DR3 & 3426281199424105472 & 92.1590 & 24.3705 & 0.29   & 3.24      & LAMOST   \\
3426290579632615040 & 92.4443 & 24.3706 & -17.92  & 12.88     & Gaia DR3 & 3426290712774774272 & 92.3949 & 24.3712 & -3.53  & 3.78      & LAMOST   \\
3426290712774762880 & 92.3947 & 24.3601 & -23.30  & 10.26     & Gaia DR3 & 3426316826173858048 & 92.4103 & 24.6761 & -2.14  & 0.64      & LAMOST   \\
3426290751432276224 & 92.4041 & 24.3783 & 2.44    & 6.25      & Gaia DR3 & 3425484427152989824 & 92.5376 & 23.8721 & -3.98  & 2.99      & LAMOST   \\
3426291881003818624 & 92.5156 & 24.4199 & -20.51  & 26.03     & Gaia DR3 & 3426160321864368640 & 92.0950 & 23.9651 & -6.92  & 3.55      & LAMOST   \\
3426292533838842112 & 92.5988 & 24.4838 & 24.07   & 28.57     & Gaia DR3 & 3426285180855324672 & 92.0402 & 24.4341 & 0.57   & 4.02      & LAMOST   \\
3426293014877394048 & 92.4853 & 24.4674 & -10.63  & 7.15      & Gaia DR3 & 3426183239809245056 & 91.7662 & 24.2244 & -8.32  & 2.31      & LAMOST   \\
3426293839511034496 & 92.3734 & 24.4174 & 0.03    & 5.39      & Gaia DR3 & 3426311745231047296 & 92.1934 & 24.5882 & -6.65  & 3.34      & LAMOST   \\
3426293946886978048 & 92.3799 & 24.4145 & -5.50   & 4.91      & Gaia DR3 & 3426297211062084608 & 92.4479 & 24.5389 & -6.19  & 0.55      & LAMOST   \\
3426294011307598592 & 92.3569 & 24.4057 & -22.93  & 6.30      & Gaia DR3 & 3426266149858654336 & 92.4288 & 24.3123 & -0.86  & 2.85      & LAMOST   \\
3426294153045407232 & 92.3720 & 24.4259 & -8.61   & 5.22      & Gaia DR3 & 3425512915672953728 & 92.3599 & 24.1853 & -1.22  & 3.00      & LAMOST   \\
3426294664142621440 & 92.3904 & 24.4737 & 0.87    & 10.30     & Gaia DR3 & 3426271509977845504 & 92.2722 & 24.4265 & -6.24  & 2.86      & LAMOST   \\
3426294668441470592 & 92.3948 & 24.4699 & -3.11   & 5.11      & Gaia DR3 & 3425540742765891200 & 92.6244 & 24.3793 & -4.59  & 2.38      & LAMOST   \\
3426294801583856384 & 92.4152 & 24.4978 & -10.74  & 7.16      & Gaia DR3 & 3425509548417900032 & 92.5815 & 24.1345 & -4.59  & 0.69      & LAMOST   \\
3426295076459482496 & 92.3533 & 24.4657 & -20.16  & 21.23     & Gaia DR3 & 3426254909924985728 & 92.1721 & 24.0516 & -4.18  & 2.10      & LAMOST   \\
3426295493075191296 & 92.3737 & 24.4905 & -25.14  & 16.20     & Gaia DR3 & 3426257212027455360 & 92.2342 & 24.1333 & -5.30  & 2.58      & LAMOST   \\
3426295905392041216 & 92.3734 & 24.5353 & -13.97  & 9.83      & Gaia DR3 & 3426327516351117056 & 91.9017 & 24.4703 & -4.24  & 0.48      & LAMOST   \\
3426296145910200576 & 92.4705 & 24.4929 & -2.88   & 9.37      & Gaia DR3 & 3426294870301054464 & 92.3412 & 24.4365 & -7.31  & 3.71      & LAMOST   \\
3426296347772102016 & 92.4685 & 24.5094 & 21.95   & 10.48     & Gaia DR3 & 3426289647622848896 & 92.4458 & 24.3406 & -5.10  & 0.50      & LAMOST   \\
3426297000604825856 & 92.5083 & 24.5662 & -1.69   & 20.63     & Gaia DR3 & 3425541464320395264 & 92.5986 & 24.4206 & -0.33  & 2.85      & LAMOST   \\
3426297069326625408 & 92.4276 & 24.5168 & -13.27  & 4.85      & Gaia DR3 & 3426265497023655936 & 92.3454 & 24.2573 & -10.03 & 1.67      & LAMOST   \\
3426297481643580288 & 92.4265 & 24.5626 & 0.15    & 12.76     & Gaia DR3 & 3426290437896838912 & 92.4275 & 24.3478 & -6.36  & 1.18      & LAMOST   \\
3426297584720378880 & 92.4596 & 24.5477 & -22.32  & 4.29      & Gaia DR3 & 3426303769475818368 & 92.5190 & 24.6167 & -28.50 & 2.09      & LAMOST   \\
3426297726458145536 & 92.4855 & 24.5723 & -23.01  & 7.75      & Gaia DR3 & 3426363589780653824 & 92.2046 & 24.8102 & -0.18  & 3.22      & LAMOST   \\
3426298512433316480 & 92.6045 & 24.5116 & 9.18    & 10.18     & Gaia DR3 & 3426282608172999552 & 92.1124 & 24.4326 & -0.21  & 3.66      & LAMOST   \\
3426298787313576192 & 92.6862 & 24.5371 & 0.47    & 7.41      & Gaia DR3 & 3426294629785093376 & 92.3809 & 24.4638 & -6.93  & 2.34      & LAMOST   \\
3426300230422739840 & 92.6422 & 24.6068 & -112.91 & 12.12     & Gaia DR3 & 3426314940686657920 & 92.2283 & 24.7115 & -7.65  & 2.10      & LAMOST   \\
3426302876120086144 & 92.5153 & 24.5811 & -2.41   & 23.02     & Gaia DR3 & 3426269822051746944 & 92.2717 & 24.3253 & -1.14  & 2.43      & LAMOST   \\
3426306934868090752 & 92.2819 & 24.4649 & -17.22  & 7.03      & Gaia DR3 & 3426256249954781312 & 92.1281 & 24.1117 & -7.99  & 3.85      & LAMOST   \\
3426307037947298304 & 92.2881 & 24.4894 & -15.35  & 12.28     & Gaia DR3 & 3426327340253767936 & 91.8739 & 24.4345 & -5.85  & 3.08      & LAMOST   \\
3426307141026510208 & 92.2903 & 24.4998 & -62.94  & 8.73      & Gaia DR3 & 3426278519364235520 & 91.9692 & 24.3340 & -5.03  & 1.18      & LAMOST   \\
3426307244105326080 & 92.2709 & 24.5011 & 8.51    & 7.36      & Gaia DR3 & 3426263362420622208 & 92.2860 & 24.1867 & -3.08  & 3.76      & LAMOST   \\
3426307274166600576 & 92.2488 & 24.5046 & -2.91   & 13.39     & Gaia DR3 & 3426270337449943936 & 92.3496 & 24.3886 & -8.58  & 1.77      & LAMOST   \\
3426307450263739776 & 92.2928 & 24.5290 & 2.17    & 10.85     & Gaia DR3 & 3425541155082750976 & 92.6500 & 24.3927 & -2.38  & 1.21      & LAMOST   \\
3426307450263744384 & 92.2751 & 24.5321 & -14.77  & 7.08      & Gaia DR3 & 3426264221414080384 & 92.2728 & 24.2191 & -4.79  & 0.79      & LAMOST   \\
3426307862580583936 & 92.3128 & 24.5479 & 6.57    & 6.86      & Gaia DR3 & 3425501538301403904 & 92.3689 & 23.9796 & -8.34  & 3.31      & LAMOST   \\
3426307927004031104 & 92.3387 & 24.5554 & -19.60  & 7.88      & Gaia DR3 & 3425505700127302144 & 92.2267 & 24.0522 & -3.38  & 0.52      & LAMOST   \\
3426308343616955392 & 92.2223 & 24.5419 & 20.74   & 8.11      & Gaia DR3 & 3425511506923033344 & 92.4092 & 24.1080 & -4.30  & 0.54      & LAMOST   \\
3426308682915870592 & 92.2861 & 24.5764 & -21.04  & 11.89     & Gaia DR3 & 3426268348881945600 & 92.2582 & 24.3176 & -12.45 & 0.60      & LAMOST   \\
3426308721574039680 & 92.3027 & 24.5684 & -22.37  & 9.17      & Gaia DR3 & 3426278618145066752 & 91.9106 & 24.3304 & -10.12 & 2.28      & LAMOST   \\
3426309477488266112 & 92.3391 & 24.5841 & 26.91   & 12.29     & Gaia DR3 & 3425540918858974976 & 92.5599 & 24.3794 & -1.49  & 4.11      & LAMOST   \\
3426310607061215488 & 92.2994 & 24.6344 & -2.73   & 18.56     & Gaia DR3 & 3426307171089700224 & 92.3154 & 24.5135 & -8.66  & 2.38      & LAMOST   \\
3426310783158295040 & 92.3804 & 24.6377 & -31.13  & 15.93     & Gaia DR3 & 3426268589400145920 & 92.1742 & 24.2845 & -4.68  & 0.80      & LAMOST   \\
3426312187609181696 & 92.2312 & 24.6179 & -19.11  & 15.96     & Gaia DR3 & 3426314047333449088 & 92.2903 & 24.6940 & -3.15  & 0.75      & LAMOST   \\
3426312226267366656 & 92.2101 & 24.6161 & -6.74   & 8.24      & Gaia DR3 & 3425512743873602176 & 92.3829 & 24.1774 & -10.84 & 0.50      & LAMOST   \\
3426312844742670848 & 92.1546 & 24.6321 & -7.25   & 7.82      & Gaia DR3 & 3426302708620191104 & 92.5781 & 24.5881 & -8.52  & 2.06      & LAMOST   \\
3426313978613974656 & 92.2937 & 24.6829 & 11.08   & 7.50      & Gaia DR3 & 3426314665808749312 & 92.2600 & 24.6879 & -2.04  & 1.90      & LAMOST   \\
3426314012973715584 & 92.2815 & 24.6871 & -14.20  & 4.63      & Gaia DR3 & 3426161863753205888 & 91.8309 & 23.9062 & -1.67  & 1.76      & LAMOST   \\
3426314837607437824 & 92.2577 & 24.7040 & -5.40   & 7.31      & Gaia DR3 & 3426285494391048576 & 92.0642 & 24.4241 & -3.97  & 0.56      & LAMOST   \\
3426328203545934848 & 91.7721 & 24.4682 & -0.39   & 9.14      & Gaia DR3 & 3426314940686657920 & 92.2238 & 24.7137 & 5.80   & 3.83      & LAMOST  
\end{tabular}%
}
\end{table}
